# Supplementary material for: de-Broglie Wavelength Enhanced Weak Equivalence Principle Test for Atoms in Different Hyperfine States
Source: arXiv:2210.08533 source file (2022-10-18)
Supplement: Supplementary file 1 [file Supplemental_material.pdf]

# Supplementary Material for “de-Broglie Wavelength Enhanced Weak Equivalence Principle Test for Atoms in Different Hyperfine States”

Yao-Yao Xu, Xiao-Bing Deng, Xiao-Chun Duan\*, Lu-Shuai Cao, Min-Kang Zhou,  
Cheng-Gang Shao, and Zhong-Kun Hu†

MOE Key Laboratory of Fundamental Quantities Measurement,  
Hubei Key Laboratory of Gravitation and Quantum Physics, School of Physics,  
Huazhong University of Science and Technology, Wuhan 430074, China

This supplemental material contains two parts. The first part provides the theoretical calculation of the gravitational-acceleration induced phase shift in a Mach-Zehnder atom interferometer if internal energy contributes differently to inertia and weight. The calculation mainly follows Ref. [S1]. The second part provides the evaluation of the disturbances due to magnetic field inhomogeneity.

## I. Theoretical calculation of the violation signal

According to mass-energy equivalence, the mass operator  $\hat{M}$  of an atom in different internal energy states can be expressed as

$$\hat{M} = m\hat{I} + \frac{\hat{H}}{c^2}, \quad (\text{S1})$$

where  $m$  denotes the mass irrelevant to the atom internal energy and  $\hat{H}$  denotes the Hamiltonian concerning only the interactions between the components constituting the atom. If inertial and gravitational mass are intentionally distinguished and internal energy may contribute differently to inertia and weight, the mass operator is then

$$\hat{M}_\alpha = m_\alpha\hat{I} + \frac{\hat{H}_\alpha}{c^2}, \quad (\text{S2})$$

where the subscript  $\alpha = \text{i, g}$  refers to inertia and weight, respectively. With these considerations, the free fall acceleration of an atom in different internal states is calculated by

$$\hat{a} = \hat{M}_g \hat{M}_i^{-1} g, \quad (\text{S3})$$

where  $g$  denotes the strength of the local gravitational field. For the two ground hyperfine states of  $^{87}\text{Rb}$  atoms which correspond to the eigenstates of the Hamiltonian  $\hat{H}_i$ , the accelerations are

$$a_j = \langle j | \hat{M}_g \hat{M}_i^{-1} | j \rangle g = \frac{m_g}{m_i} r_j g, \quad (\text{S4})$$

where  $j = 1, 2$  specifies the corresponding hyperfine states. In Eq. (S4), parameters  $r_j$  ( $j = 1, 2$ ) are introduced, which are calculated from  $\hat{M}_g \hat{M}_i^{-1}$  with the approximation of keeping only the lowest order in  $1/c^2$  as in Ref. [S1]. The parameters are explicitly written as

$$r_j = 1 + \frac{\langle j | \hat{H}_g | j \rangle}{m_g c^2} - \frac{\langle j | \hat{H}_i | j \rangle}{m_i c^2}. \quad (\text{S5})$$

The difference of the free fall accelerations for an atom in different hyperfine states thus yields the Eötvös ratio, namely

$$\eta = 2 \times \frac{a_2 - a_1}{a_2 + a_1} = 2 \times \frac{\langle 2 | \hat{M}_g \hat{M}_i^{-1} | 2 \rangle - \langle 1 | \hat{M}_g \hat{M}_i^{-1} | 1 \rangle}{\langle 2 | \hat{M}_g \hat{M}_i^{-1} | 2 \rangle + \langle 1 | \hat{M}_g \hat{M}_i^{-1} | 1 \rangle} \approx r_2 - r_1, \quad (\text{S6})$$

where the approximation of  $r_j \approx 1$  is considered. According to Eq. (S6), the validation of the weak equivalence principle (WEP) requires  $r_1 = r_2$ . In Eq. (S2), there is possible difference for internal energy contributing to inertia and weight, causing  $r_j \neq 1$ . If we further considered that the difference may vary with different hyperfine states, we may find that  $r_1 \neq r_2$ , causing the violation of WEP. The above discussion considers the WEP violation mechanism that internal energy may contribute differently to inertia and weight. Actually, one can also start from the expression of  $a_j = (m_g / m_i) r_j g$  ( $j = 1, 2$ ) to account for other WEP violation mechanisms. For example, spin-dependent interactions [S2] may also lead to  $r_1 \neq r_2$ , causing the violation of WEP for atoms in different hyperfine states.

Possible WEP violation for atoms in different hyperfine states is then incorporated into a typical Mach-Zehnder atom interferometer based on two-photon Raman stimulated transition which is usually used to measure the gravitational acceleration. Considering a homogeneous gravitational field, the Hamiltonian for an atom during the free evolution time can be expressed as

$$\hat{H} = \hat{M}_i c^2 + \hat{M}_i^{-1} \frac{\hat{p}^2}{2} + g(\hat{M}_g \hat{M}_i^{-1}) \hat{M}_i \hat{z}, \quad (\text{S7})$$

where  $\hat{p}$  and  $\hat{z}$  are the momentum and position operators of the atom, respectively. Here only the vertical dimension is considered. According to Eq. (S4) with the off-diagonal elements of  $\hat{M}_g \hat{M}_i^{-1}$  further neglected, the Hamiltonian is approximated as

$$\hat{H} = \hat{M}_i c^2 + \hat{M}_i^{-1} \frac{\hat{p}^2}{2} + \left( \frac{m_g}{m_i} \right) g \begin{bmatrix} r_1 \\ r_2 \end{bmatrix} \hat{M}_i \hat{z}. \quad (\text{S8})$$

We note that  $\langle 2 | \hat{M}_i | 2 \rangle - \langle 1 | \hat{M}_i | 1 \rangle = h\nu_0 / c^2$ , where  $\nu_0$  is the clock transition frequency between the two ground hyperfine states of  $^{87}\text{Rb}$  atoms. The phase shift proportional to  $h\nu_0 / mc^2$  is much smaller than 1 mrad with our typical experimental parameters, and thus is neglected (our aimed uncertainty of measuring the phase shift is at mrad level).

The phase shift of a Raman Mach-Zehnder Interferometer (MZI) can be divided into three parts, the phase shift due to free evolution between the Raman pulses (denoted as  $\Delta\varphi_{\text{free}}$ ), the phase shift due to the interaction with the Raman pulses (denoted as  $\Delta\varphi_{\text{laser}}$ ), and the phase shift due to possible separation of the trajectories along the two arms (denoted as  $\Delta\varphi_{\text{sep}}$ ). The free evolution phase shift is calculated as  $\Delta\varphi_{\text{free}} = \int L dt / \hbar$ , where  $L$  stands for the Lagrangian and the integral is along the trajectory over each arm. The phase shift due to the interaction with the Raman pulses is calculated as  $\Delta\varphi_{\text{laser}} = \vec{k}_L^{\text{eff}} (\vec{z}_A - \vec{z}_B - \vec{z}_{B'} - \vec{z}_C)$ , where  $\vec{k}_L^{\text{eff}}$  is the usual wave vector of Raman laser, and the positions have been labeled in Fig. S1. The phase shift due to

the separation is calculated as  $\Delta\phi_{\text{sep}} = -m_i V(z_C - z_{C'}) / \hbar$ , where  $V$  is the velocity of the atoms at the exit of the interferometer.

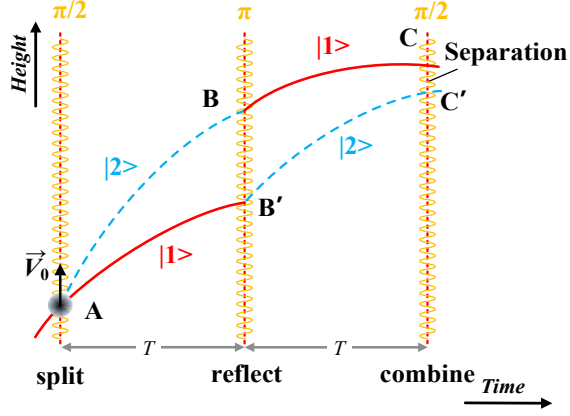

Fig. S1 A Mach-Zehnder atom interferometer where the two branches don't close.

The final total phase shift is

$$\Delta\phi = -(r_2 - r_1)(\vec{k}_m^{\text{eff}} \cdot \hat{g}) \left( \frac{m_g}{m_i} \right) gT^2 + r_1(\vec{k}_L^{\text{eff}} \cdot \hat{g}) \left( \frac{m_g}{m_i} \right) gT^2, \quad (\text{S9})$$

where  $\hat{g}$  is the direction of local gravitational acceleration. And  $\vec{k}_m^{\text{eff}} \equiv m_i \vec{V}_\pi / \hbar$  stands for the wave vector of matter wave, where  $\vec{V}_\pi = \vec{V}_0 + \frac{r_1 + r_2}{2} \left( \frac{m_g}{m_i} \right) gT \hat{g}$  denotes the velocity of the atom at the reflecting  $\pi$  pulse ( $\vec{V}_0$  is the atom velocity at the entrance of the interferometer).

During the calculation of  $\Delta\phi$ , both the free evolution phase shift and the separation phase shift are related to the de-Broglie wavelength, contributing to the WEP test signal. For comparison, in a Raman MZI with a linear gravity gradient present, the free evolution phase shift is

$$\Delta\phi_{\text{free}} = k_L^{\text{eff}} \gamma T^3 \left( V_0 + \frac{V_r}{2} - 2gT \right), \quad (\text{S10})$$

and the separation phase shift is

$$\Delta\phi_{\text{sep}} = -\frac{m_i (V_0 + V_r - 2gT)}{\hbar} \Delta z = -k_L^{\text{eff}} \gamma T^3 (V_0 + V_r - 2gT), \quad (\text{S11})$$

where  $\gamma$  denotes the strength of gravity gradient,  $V_r$  is then recoil velocity, and the

separation  $\Delta z = \gamma V_r T^3$  is substituted. According to Eq. (S10) and Eq. (S11), the free evolution phase shift and the separation phase shift nearly cancel when a linear gravity gradient is considered, although the two phase shifts are both related to the de-Broglie wavelength individually. But the situation is different for the WEP test, where the phase shifts dependent on the de-Broglie wavelength in  $\Delta\phi_{\text{free}}$  and  $\Delta\phi_{\text{sep}}$  do not cancel, especially for large  $V_0$ . The difference between the two situations is originated from that the gravity gradient is the same for the atom in each hyperfine state while the free fall acceleration is considered to be hyperfine-state dependent for the WEP test.

A common-mode measurement by reversing  $\hat{k}_L^{\text{eff}}$  (the direction of  $\vec{k}_L^{\text{eff}}$ ) is applied to extract out the WEP test signal from the total phase shift. With a gravity gradient  $\frac{m_g}{m_i} r_j \gamma$  present for each hyperfine states and considering the finite light speed

effect [S3], the phase shift for the common-mode measurement is

$$\Delta\Phi_c = \frac{1}{2} k_L^{\text{eff}} r_1 \left( \frac{m_g}{m_i} \right) \gamma V_r T^3 + \frac{m_i V_\pi}{\hbar} (r_2 - r_1) T^2 \left\{ \left( \frac{m_g}{m_i} \right) g - \left( \frac{m_g}{m_i} \right) \gamma \left[ z_0 + V_0 T - \frac{3}{4} \left( \frac{m_g}{m_i} \right) g T^2 \right] \right\} - 2\alpha_L V_\pi T^2 / c, \quad (\text{S12})$$

where  $c$  denotes the light speed, and  $\alpha_L$  is the chirp rate of the effective frequency of the Raman laser for  $k_L^+$ . In Eq. (S12), the residual phase shift due to normal gravity is not listed.

## II. Evaluation of the disturbance due to magnetic field inhomogeneity

As disturbances dependent on  $\hat{k}_L^{\text{eff}}$  in usual gravity measurements are suppressed by the common-mode measurement here, disturbances independent on  $\hat{k}_L^{\text{eff}}$  contribute to the major errors for our WEP test. In order to obtain a big value of  $V_\pi$ , the position of the atom cloud deviates far away from the apex of the fountain at the moment applying the interfering  $\pi$  pulse. This configuration results in a significant disturbance originating from the magnetic field inhomogeneity, even though atoms are prepared in

$m_F = 0$ . The corresponding disturbance induced by the second Zeeman shift is quadratic in the injection current  $I$  for the bias coil [S4], which is expressed as

$$\Delta\phi_B = \Delta\phi_0 + \xi \cdot I + \beta \cdot I^2, \quad (\text{S13})$$

where  $\xi$  is the first order coefficient and  $\beta$  is the second order coefficient.  $\xi$  and  $\beta$  both generally depend on the trajectory of the atoms during the interference and the detail parameters of the bias coil.  $\Delta\phi_0$  is the part dependent on the residual magnetic field  $B_0$  but independent on the injection current  $I$ . Here  $\Delta\phi_B$  is divided into the current dependent and independent parts, and the two parts are determined individually using different methods. In order to evaluate the current dependent part of  $\Delta\phi_B$ , the injection current  $I$  is modulated from 15 mA to 90 mA with a step of 15 mA for each direction of  $\vec{k}_L^{\text{eff}}$ . The corresponding variation of the phase shift is recorded, which is shown in Fig. S2. A quadratic polynomial fit is performed to obtain the values of  $\xi$  and  $\beta$ . Then the current dependent part of  $\Delta\phi_B$  can be calculated by  $\xi \cdot I + \beta \cdot I^2$ . We note that the intercept of the vertical axis for the quadratic polynomial fit has never been used in the evaluation of  $\Delta\phi_B$ .

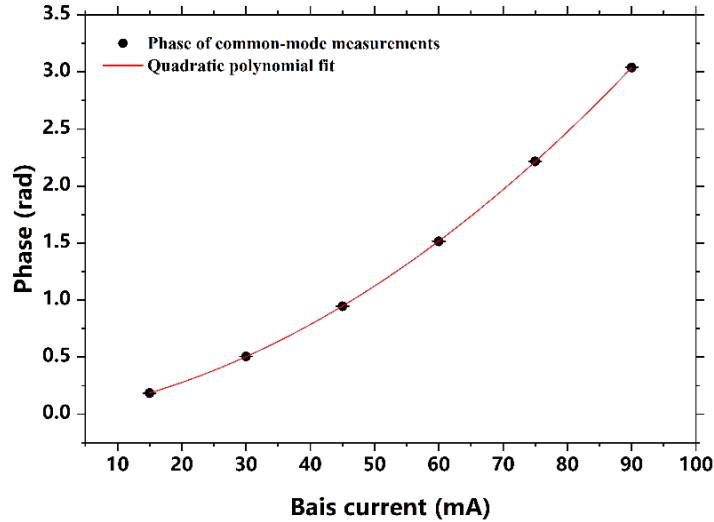

Fig. S2 Variation of the common-mode measurements versus the injection current in the bias coil. A quadratic polynomial fitting result is displayed as the red line.

For the evaluation of  $\Delta\phi_0$ , the magnetic field along the interference tube is mapped by the magnetic sensitive Raman spectroscopy in different injection currents. And for each space position, the measurements of the magnetic field with different

injection currents are fitted linearly, educing the intercept as the residual magnetic field  $B_0$  at this position. The obtained profile of the residual magnetic field is as shown in Fig. S3, which is then used to determine  $\Delta\phi_0$  by theoretical calculation as

$$\Delta\phi_0 = \kappa \int_0^T B_0^2 dt - \kappa \int_{-T}^0 B_0^2 dt, \quad \text{Eq. (S14)}$$

where  $\kappa=2\pi \cdot 575.15 \text{ Hz/G}^2$  is the second order Zeeman coefficient. Substituting the residual magnetic field shown in Fig. (S3),  $\Delta\phi_0$  is determined as 4.6(3) mrad.

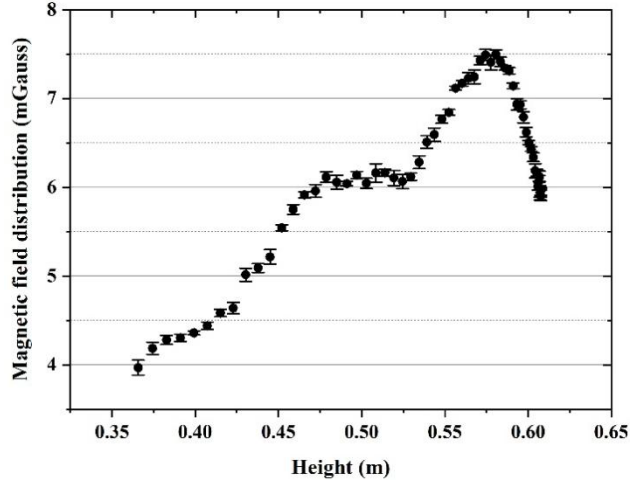

Fig. S3 The profile of the residual magnetic field  $B_0$  with  $I=0$  A.

In principle,  $\Delta\phi_B$  can be calculated directly using the mapped magnetic field distribution at  $I=15$  mA. However, the contribution of the magnetic field measurement uncertainty is proportional to the absolute value of the magnetic field since the Zeeman effect is quadratic for atoms in magnetic insensitive sublevels. In our experiment,  $B_0$  is about 7(1) mG, about 26 times smaller than the bias magnetic field at  $I=15$  mA. The magnetic field measurement uncertainty only affects the calculation of  $\Delta\phi_0$  where the absolute value of the magnetic field is the small residual magnetic field  $B_0$ . Meanwhile, the current dependent part of  $\Delta\phi_B$  is determined precisely by the current modulation experiment. The final contribution due to the Zeeman effect is evaluated to be 192(3) mrad, where the correction uncertainty mainly comes from the fitting uncertainty of  $\xi$ .

## Reference

[S1] G. Rosi, G. D'Amico, L. Cacciapuoti, et. al., Quantum test of the equivalence

principle for atoms in coherent superposition of internal energy states, Nat. Commun. **8**, 15529 (2017).

[S2] D. J. Wineland, J. J. Bollinger, D. J. Heinzen, et. al., Search for anomalous spin-dependent forces using stored-ion spectroscopy, Phys. Rev. Lett. **67**, 1735 (1991).

[S3] Yu-Jie Tan, Cheng-Gang Shao, and Zhong-Kun Hu, Finite-speed-of-light perturbation in atom gravimeters, Phys. Rev. A **94**, 013612 (2016).

[S4] A. Peters, K. Y. Chung, and S. Chu, Metrologia **38**, 25 (2001).
